# Supplementary material for: A2BFR: Attribute-Aware Blind Face Restoration
Source: arXiv:2603.29423 source file (2026-03-31)
Supplement: Supplementary file 1 [file X_suppl.tex]

% \clearpage
% \setcounter{page}{1}
% In this supplementary material, Sec.~\ref{sec:dataset} presents additional details of our proposed AttrFace-90K. Sec.~\ref{sec:implementary} provides the implementation details of the proposed \textbf{A$^\text{2}$BFR}. Sec.~\ref{sec:experiment} shows additional ablation study on the parameters in AAL, SDT, and CFG scales.
% Sec.~\ref{sec:userstudy} outlines the design and outcomes of our user study, further illustrating the superior performance of the proposed model.
% Sec.~\ref{sec:eval} details our Qwen3-VL evaluation process and provides additional results.Sec.~\ref{sec:qualitative} provides additional qualitative comparisons to further demonstrate the superiority of \textbf{A$^\text{2}$BFR}. Finally, Sec.~\ref{sec:limitation} discusses the limitations of our method and outlines future work. 

In this supplementary material, Sec.~\ref{sec:dataset} presents additional details of our proposed AttrFace-90K. Sec.~\ref{sec:implementary} provides the implementation details of the proposed \textbf{A$^\text{2}$BFR}. Sec.~\ref{sec:experiment} shows additional ablation studies on the parameters in AAL, SDT, and CFG scales.
Sec.~\ref{sec:userstudy} outlines the design and outcomes of our user study, further illustrating the superior performance of the proposed model. 
Sec.~\ref{sec:qualitative} provides additional qualitative comparisons to further demonstrate the strong performance of \textbf{A$^\text{2}$BFR}.
Finally, Sec.~\ref{sec:limitation} discusses the limitations of our method and outlines future work. 

\section{Dataset Details}
\label{sec:dataset}

\subsection{Attribute Editing}
To address the over-editing and identity drift in the original FlowEdit~\cite{kulikov2025flowedit}, we incorporate a hyperparameter $\alpha$ into our algorithm, which interpolates between the original and edited noise maps to balance semantic modification with structural preservation.

\begin{wrapfigure}{r}{0.6\columnwidth}
\vspace{-0.8em}
\begin{minipage}{0.58\columnwidth}
\small
\hrule
\vspace{0.3em}
\refstepcounter{algocf}
\textbf{Algorithm \thealgocf} Simplified algorithm for FlowEdit-$\alpha$\label{alg:flowedit_mod}
\vspace{-0.3em}
\hrule
\vspace{0.4em}

\textbf{Input:} Real image $X^{\mathrm{src}}_0$, time steps $\{t_i\}_{i=0}^{T}$, maximum step index $n_{\max}$

\textbf{Output:} Edited image $X^{\mathrm{tar}}_0$

\textbf{Init:} $Z^{\mathrm{FE}}_{t_{\max}} \leftarrow X^{\mathrm{src}}_0$

\textbf{for} $i \leftarrow n_{\max}$ \textbf{downto} $1$ \textbf{do}

\quad $V^{\mathrm{noise}}_{t_i} \leftarrow V^{\mathrm{src}}(Z^{\mathrm{src}}_{t_i}, t_i)$

\quad $Z^{\mathrm{src}}_{t_{i-1}} \leftarrow Z^{\mathrm{src}}_{t_i} - (t_{i-1}-t_i)V^{\mathrm{noise}}_{t_i}$

\textbf{end for}

$N_{\mathrm{initial}} \leftarrow Z^{\mathrm{src}}_{1}$

\textbf{for} $i \leftarrow n_{\max}$ \textbf{downto} $1$ \textbf{do}

\quad Sample Gaussian noise $N_{t_i} \sim \mathcal{N}(0,1)$

\quad $Z^{\mathrm{src}}_{t_i} \leftarrow (1-t_i)X^{\mathrm{src}} + \textcolor{red}{\alpha t_i N_{t_i} + (1-\alpha)t_i N_{\mathrm{initial}}}$

\quad $Z^{\mathrm{tar}}_{t_i} \leftarrow Z^{\mathrm{FE}}_{t_i} + Z^{\mathrm{src}}_{t_i} - X^{\mathrm{src}}$

\quad $V^{\Delta}_{t_i} \leftarrow V^{\mathrm{tar}}(Z^{\mathrm{tar}}_{t_i}, t_i) - V^{\mathrm{src}}(Z^{\mathrm{src}}_{t_i}, t_i)$

\quad $Z^{\mathrm{FE}}_{t_{i-1}} \leftarrow Z^{\mathrm{FE}}_{t_i} + (t_{i-1}-t_i)V^{\Delta}_{t_i}$

\textbf{end for}

\textbf{return} $Z^{\mathrm{FE}}_0 = X^{\mathrm{tar}}_0$

\vspace{0.4em}
\hrule
\end{minipage}
\vspace{-1.0em}
\end{wrapfigure}

As outlined in Algorithm~\ref{alg:flowedit_mod}, our method replaces the original FlowEdit by linearly interpolating between the random noise \(N_{t_i}\) and the initial noise \(N_{\text{initial}}\) for explicit control over the edit. We ultimately adopted this design because the substantial improvement in output fidelity justifies the 1.5x increase in computational time.

Quantitative and qualitative results are shown in Table~\ref{Tab:alpha_ae} and Figure~\ref{fig:alpha_ae}. $\alpha =0.85$ was selected as the adopted setting for dataset construction, as it achieves an optimal balance between editability and facial identity preservation.

\begin{figure}[t]
    \centering
    \includegraphics[width=0.9\columnwidth]{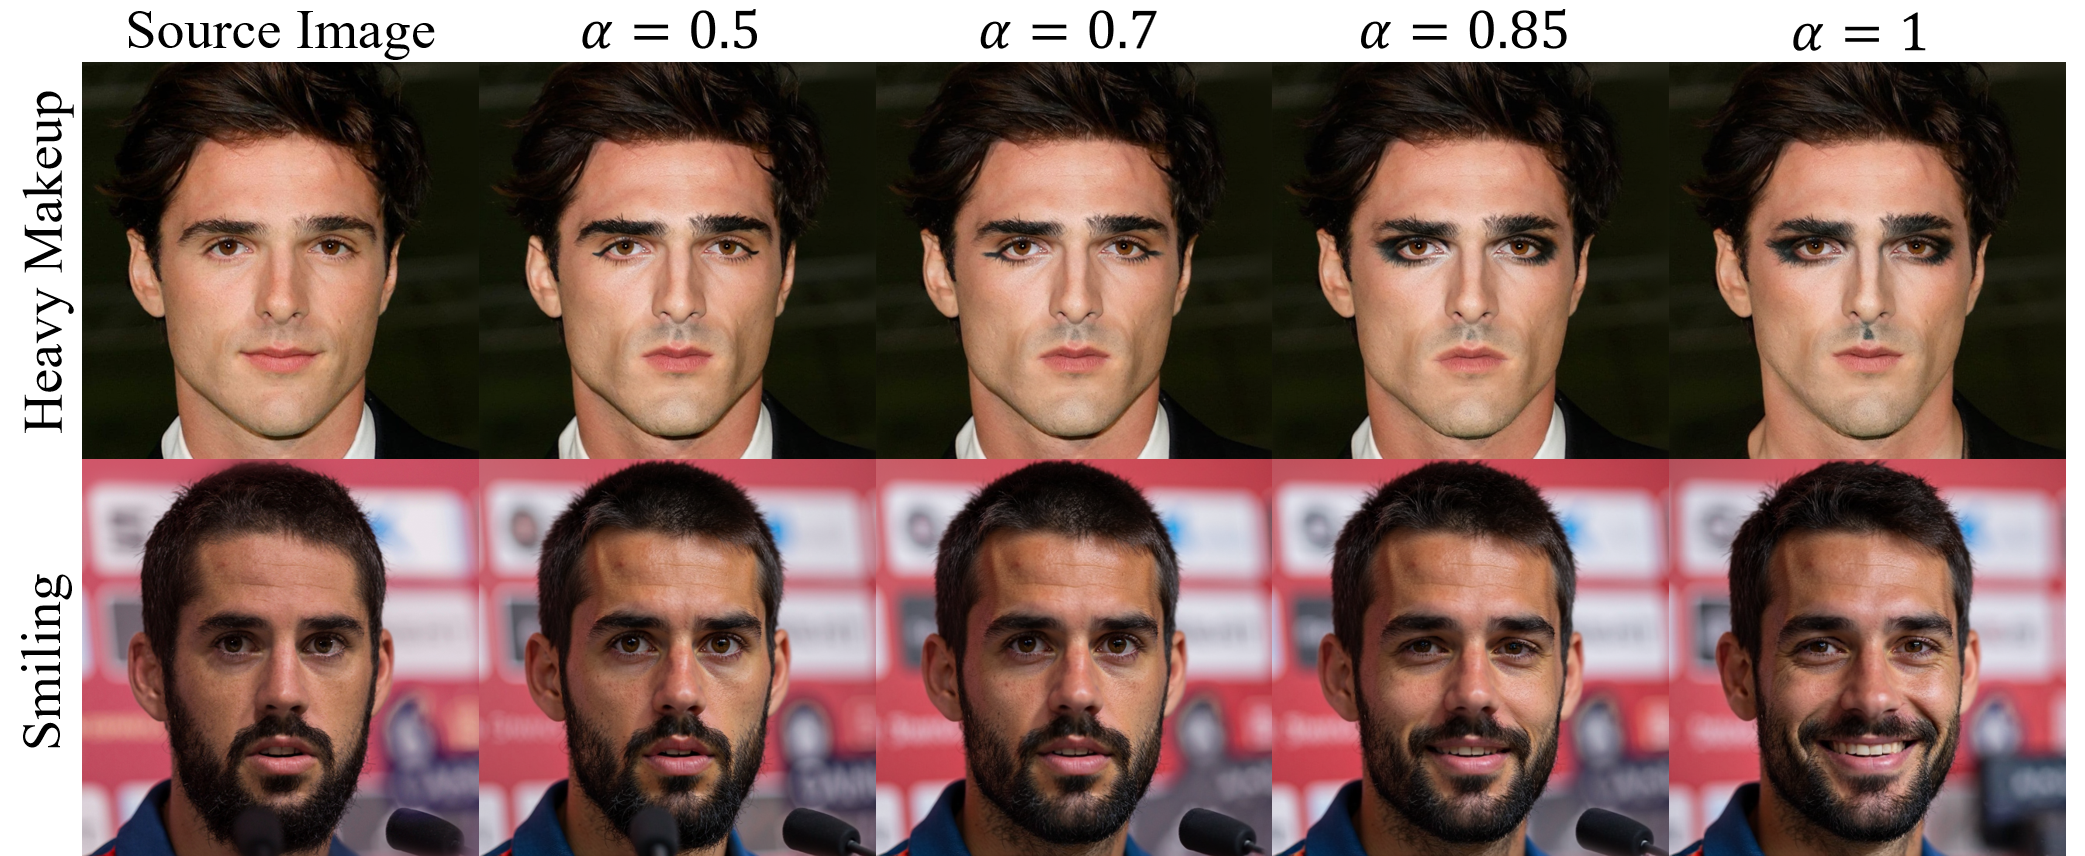}
    \caption{Qualitative results of Attribute Editing. As $\alpha$ approaches 1, fidelity decreases while the target attribute becomes more pronounced. }
    \label{fig:alpha_ae}
    \vspace{-5pt}
\end{figure}

\begin{table}[t]
  \caption{Quantitative comparison of different $\alpha$ on a subset of AttrFace-90K.}
  \centering
% 缩小到85%
    \begin{tabular}{l c c c c}
      \toprule  
      Metrics & $\alpha{=}0.5$ & $\alpha{=}0.7$ & $\alpha{=}0.85$ & $\alpha{=}1$ \\
      \midrule
      AA$\uparrow$ & 0.6167 & 0.6417 & 0.7167 & 0.7500 \\
      ID-Sim$\uparrow$ & 0.6713 & 0.6695 & 0.6532 & 0.6214 \\
      \bottomrule
    \end{tabular}
  
  \label{Tab:alpha_ae}
\end{table}
\vspace{-10pt}

\subsection{Quality Control for AttrFace-90K}
% 在得到编辑图像之后，我们使用了一套严格的post check方法来control AttrFace-90K的质量。我们对编辑图像进行三阶段的筛查：首先，我们使用与Prompt Construction中相同的方式，评估属性的置信度。我们筛去所有属性置信度小于0.6的图片，以保证编辑所的图片中该属性为positive. 随后，我们对编辑图片与原始图片检测它们的Arcface ID相似度，筛去所有ID 相似度小于0.5 的图片，以保证数据集中图片对的身份一致性。最后，我们筛去了所有LPIPS 小于0.3的图片，以保证编辑前后的感知一致性。
% 通过上述检查....

% Following the attribute editing procedure, we established a rigorous three-tier quality assessment protocol to ensure the integrity of the AttrFace-90K dataset. First, attribute confidence scores were evaluated using the same methodology applied during prompt construction, with all images scoring below 0.6 excluded to guarantee reliable attribute manifestation. Second, we computed ArcFace~\cite{deng2019arcface} identity similarity between edited and original images, systematically discarding pairs demonstrating similarity scores below 0.5 to preserve identity consistency. Finally, image pairs exhibiting LPIPS values higher than 0.3 were removed to maintain adequate perceptual similarity between source and edited images. Finally, we apply manual check to ensure the overall quality. Subsequently, we regenerated the textual descriptions $T^\text{tar}$ following the identical prompt construction pipeline detailed in the main manuscript. 

We implemented a rigorous multi-stage quality control pipeline to ensure the reliability of the AttrFace-90K dataset. First, attribute confidence was assessed using the same procedure adopted for prompt construction, and samples with scores below 0.6 were discarded to ensure clear and reliable attribute expression. Second, we measured ArcFace~\cite{deng2019arcface} identity similarity between the edited and original images, and removed pairs with similarity scores below 0.5 to preserve identity consistency. Third, we filtered out image pairs with LPIPS values greater than 0.3 to maintain adequate perceptual similarity between the source and edited images. These thresholds were determined based on pilot experiments and manual inspection of a candidate subset, with the goal of balancing attribute validity, identity preservation, and perceptual consistency. Finally, we performed manual inspection to further ensure the overall quality of the dataset. After quality filtering, we regenerated the textual descriptions $T^\text{tar}$ using the same prompt construction pipeline described in the main manuscript.

Our rigorous quality control yielded a high-quality dataset where each image pair faithfully exhibits: (1) the target attribute difference, (2) preserved identity, and (3) controlled perceptual differences. This pipeline provides a robust foundation for developing and evaluating attribute-aware face restoration models.

\subsection{More Examples of AttrFace-90K}
\begin{figure*}[t]
    \centering
    \includegraphics[width=\textwidth]{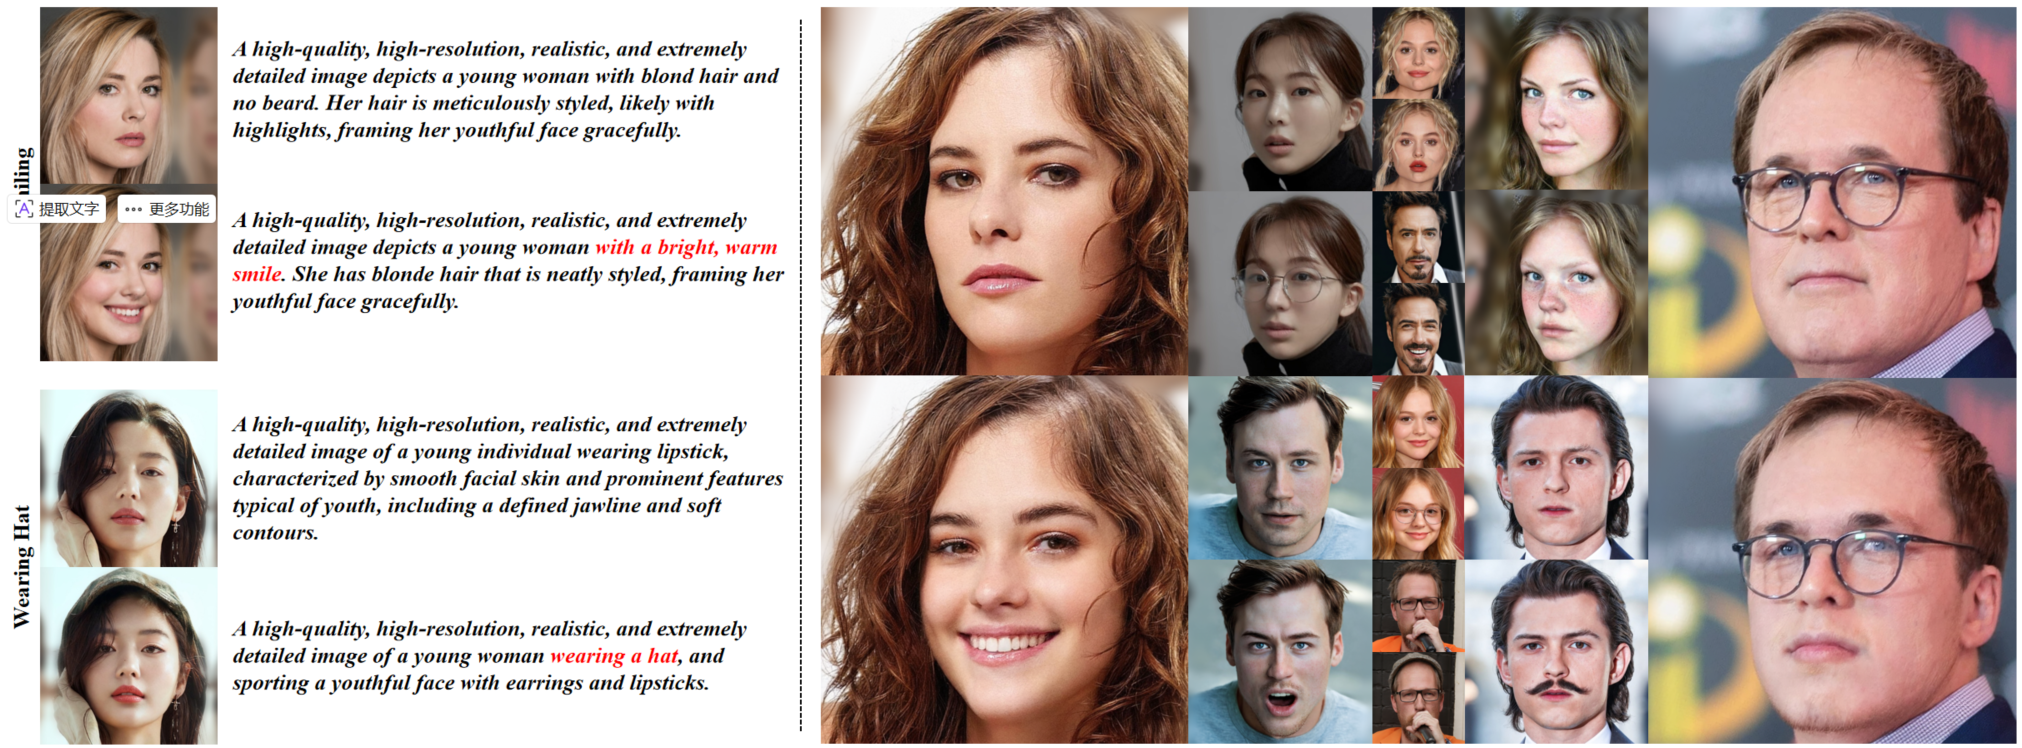}
 \vspace{-10pt}
    \caption{\textbf{Left:} Examples of $(I^\text{src}_{\text{GT}}, T^\text{src})$ and $(I^\text{tar}_{\text{GT}}, T^\text{tar})$ in AttrFace-90K.
\textbf{Right:} A quick view of AttrFace-90K.}
    \label{fig:attrface}
     %\vspace{-16pt}
     \vspace{-10pt}
\end{figure*}

The AttrFace-90K dataset comprises about 90,000 face image pairs. Each pair includes two images along with their corresponding textual captions, which are denoted as $(I^\text{src}_{\text{GT}}, T^\text{src})$ and $(I^\text{tar}_{\text{GT}}, T^\text{tar})$ in our paper, as shown in Figure~\ref{fig:attrface}. Additionally, the two images within each pair exhibit a distinct difference in a specific attribute, which is annotated in our dataset.

\section{Implementation Details}
\label{sec:implementary}

\textbf{LQ Construction} During training and fine-tuning, LQ images are synthesized online following a common degradation model expressed in Eq.~\ref{tab:degrade}, 

\begin{equation}
I_{LQ} = \left[ (I_{HQ} \ast k_{\sigma}) \downarrow_r + n_{\delta} \right]_{\text{JPEG}_q}
\label{tab:degrade}
\end{equation}
where $k_{\sigma}$ represents a blur kernel randomly selected from Gaussian blur, average blur, median blur, or motion blur, $\downarrow_r$ denotes downsampling scale, $n_{\delta}$ represents additive Gaussian noise, and $\text{JPEG}_q$ indicates JPEG compression.
To increase the severity of degradation, the downsampling ratio $r$ is set to 16, producing LQ images of $32 \times 32$ pixels. 

During the testing phase, for both the AttrFace-90K-Test and CelebRef-HQ-Test datasets, LQ images are generated following the identical degradation pipeline and remain fixed throughout all testing procedures.

\section{Additional Experiments}  % 修正拼写
\label{sec:experiment}  % 修正拼写
We introduce additional ablation studies of \textbf{A$^\text{2}$BFR} in this section.
\subsection{Effect of $\lambda$ for AAL}
To evaluate the effect of $\lambda$ in the Attribute-Aware Learning (AAL), we fixed $\alpha = 0.2$ and systematically varied $\lambda = {\{0, 0.1, 0.2, 0.5, 0.8\}}$, training separate LoRA modules for each configuration. 

As shown in Table~\ref{Tab: AAL}, increasing $\lambda$ produces a consistent improvement in SC (Semantic Consistency). This outcome aligns with theoretical expectations, as AAL provides semantic supervision that anchors the denoising trajectory to an attribute-aware embedding space, and our prompts are conditioned on these semantic embeddings. Furthermore, compared to the baseline ($\lambda=0$), enabling AAL improves semantic consistency and generally benefits overall performance, demonstrating the effectiveness of our proposed AAL.
\begin{table}[t]
  \caption{Quantitative comparison of different $\lambda$ for AAL on the subset of AttrFace-90K-Test datasets. \textbf{Best} and \underline{second best} performance are highlighted}
  \centering
  \setlength{\tabcolsep}{4pt}
  \small
  \resizebox{0.7\columnwidth}{!}{
  \begin{tabular}{l c c c c}
    \toprule  
    & \multicolumn{2}{c}{Attribute} & \multicolumn{1}{c}{Fidelity} & Quality \\
    \cmidrule(lr){2-3} \cmidrule(lr){4-4} \cmidrule(l){5-5}
    Methods/Metrics
    & SC $\uparrow$ & AA $\uparrow$
    & LPIPS $\downarrow$  & HyperIQA $\uparrow$ \\
    \midrule
    $\lambda=0$  & 94.46               & 0.6417                 & 0.2889                                      & 0.7829 \\
    $\lambda=0.1$ & 94.68                  & 0.8279                 & 0.2916                                      & 0.7773 \\
    $\lambda=0.2$ & 94.70        &  \textbf{0.8536}     & \underline{0.2863}      & \underline{0.7908} \\
    $\lambda=0.5$ & \underline{94.72}                  & 0.8369                 & \textbf{0.2858}                                        & 0.7819 \\
    $\lambda=0.8$ & \textbf{94.74}                  & \underline{0.8452}                 & 0.2933                                         & \textbf{0.7919} \\
    \bottomrule
  \end{tabular}
  }
  \label{Tab: AAL}
\end{table}

\subsection{Effect of $\alpha$ for SDT}
To evaluate the effect of $\alpha$ on SDT, we fixed $\lambda = 0.2$ and tested several values of $\alpha = \{0, 0.1, 0.2, 0.5, 0.8\}$. For each value, we trained a LoRA module and evaluated its performance on  AttrFace-90K-Test.

\begin{table}[t]
  \caption{Quantitative comparison of different $\alpha$ for SDT on the subset of AttrFace-90K-Test datasets. \textbf{Best} and \underline{second best} performance are highlighted.}
  \centering
  \setlength{\tabcolsep}{4pt}
  \small
  \resizebox{0.7\columnwidth}{!}{
  \begin{tabular}{l c c c c c}
    \toprule  
    & \multicolumn{2}{c}{Attribute} & \multicolumn{1}{c}{Fidelity} & Quality \\
    \cmidrule(lr){2-3} \cmidrule(lr){4-4} \cmidrule(l){5-5}
    Methods/Metrics
    & SC $\uparrow$ & AA $\uparrow$
    & LPIPS $\downarrow$ & HyperIQA $\uparrow$ \\
    \midrule
    $\alpha=0$ & \underline{94.77}                  & 0.7757                 & 0.2926                                   & 0.7872 \\
    $\alpha=0.1$ & 94.68                  & 0.8452                & 0.2913                                      & \underline{0.7899}  \\
    $\alpha=0.2$ & 94.70        & 0.8536     & \underline{0.2863}     & \textbf{0.7908} \\
    $\alpha=0.5$ & 94.72                  & \underline{0.8619}                 & \textbf{0.2861}                                     & 0.7808 \\
    $\alpha=0.8$ & \textbf{94.78}                  & \textbf{0.8786}                 & 0.2874                       & 0.7823 \\
    \bottomrule
  \end{tabular}
  }
  \label{Tab:SDT}
\end{table}

As shown in Table~\ref{Tab:SDT}, increasing $\alpha$ consistently improves Attribute Accuracy (AA). This trend aligns with our theoretical framework, since the $\mathcal{L}_{\text{dual}}$ term in SDT explicitly maximizes the semantic divergence between outputs generated from different textual prompts for the same degraded input. Moreover, compared to the baseline ($\alpha=0$), activating $\mathcal{L}_{\text{dual}}$ achieves substantial gains in AA and competitive performance on the other metrics, validating the efficacy of our loss design.

\subsection{Effect of CFG Scale}
We set the CFG scale to $\{1.0, 3.5, 5.5, 7.5, 10.5\}$ to evaluate the effect of CFG Scales~\cite{ho2022classifier}.

\begin{table}[t]
  \caption{Quantitative comparison of different CFG scale on the subset of AttrFace-90K-Test datasets. \textbf{Best} and \underline{second best} performance are highlighted}
  \centering
  \setlength{\tabcolsep}{4pt}
  \small
  \resizebox{0.7\columnwidth}{!}{
  \begin{tabular}{l c c c c }
    \toprule  
    & \multicolumn{2}{c}{Attribute} & \multicolumn{1}{c}{Fidelity} & Quality \\
    \cmidrule(lr){2-3} \cmidrule(lr){4-4} \cmidrule(l){5-5}
    Methods/Metrics
    & SC $\uparrow$ & AA $\uparrow$
    & LPIPS $\downarrow$ & HyperIQA $\uparrow$ \\
    \midrule
    $CFG=1.0$ & 94.34 & 0.6833 & 0.2973  & 0.6447 \\
    $CFG=3.5$ & \textbf{94.84} & 0.8167 & \textbf{0.2843}  & 0.7876 \\
    $CFG=5.5$ & 94.70 & \textbf{0.8536} & \underline{0.2863}  & \textbf{0.7908} \\
    $CFG=7.5$ & \underline{94.76} & 0.8083 & 0.2939  & 0.7893 \\
    $CFG=10.5$ & 94.73 & \underline{0.8333} & 0.2944  & \underline{0.7886} \\
    \bottomrule
  \end{tabular}
  }
  \label{Tab:CFG_ablation}
\end{table}

As shown in Table~\ref{Tab:CFG_ablation}, increasing the CFG scale from 1.0 to 5.5 enhances attribute control, with AA peaking at 0.8536, and overall image quality (HyperIQA) reaching an optimum of 0.7908, albeit at the cost of a slight reduction in structural fidelity. A trade-off in fidelity metrics is observed, where CFG=3.5 achieves the best perceptual similarity (lowest LPIPS), while higher scales compromise structural preservation.

\section{User Study}
\begin{figure*}[htbp]
    \centering
    \vspace{-8pt}
    \includegraphics[width=\textwidth]{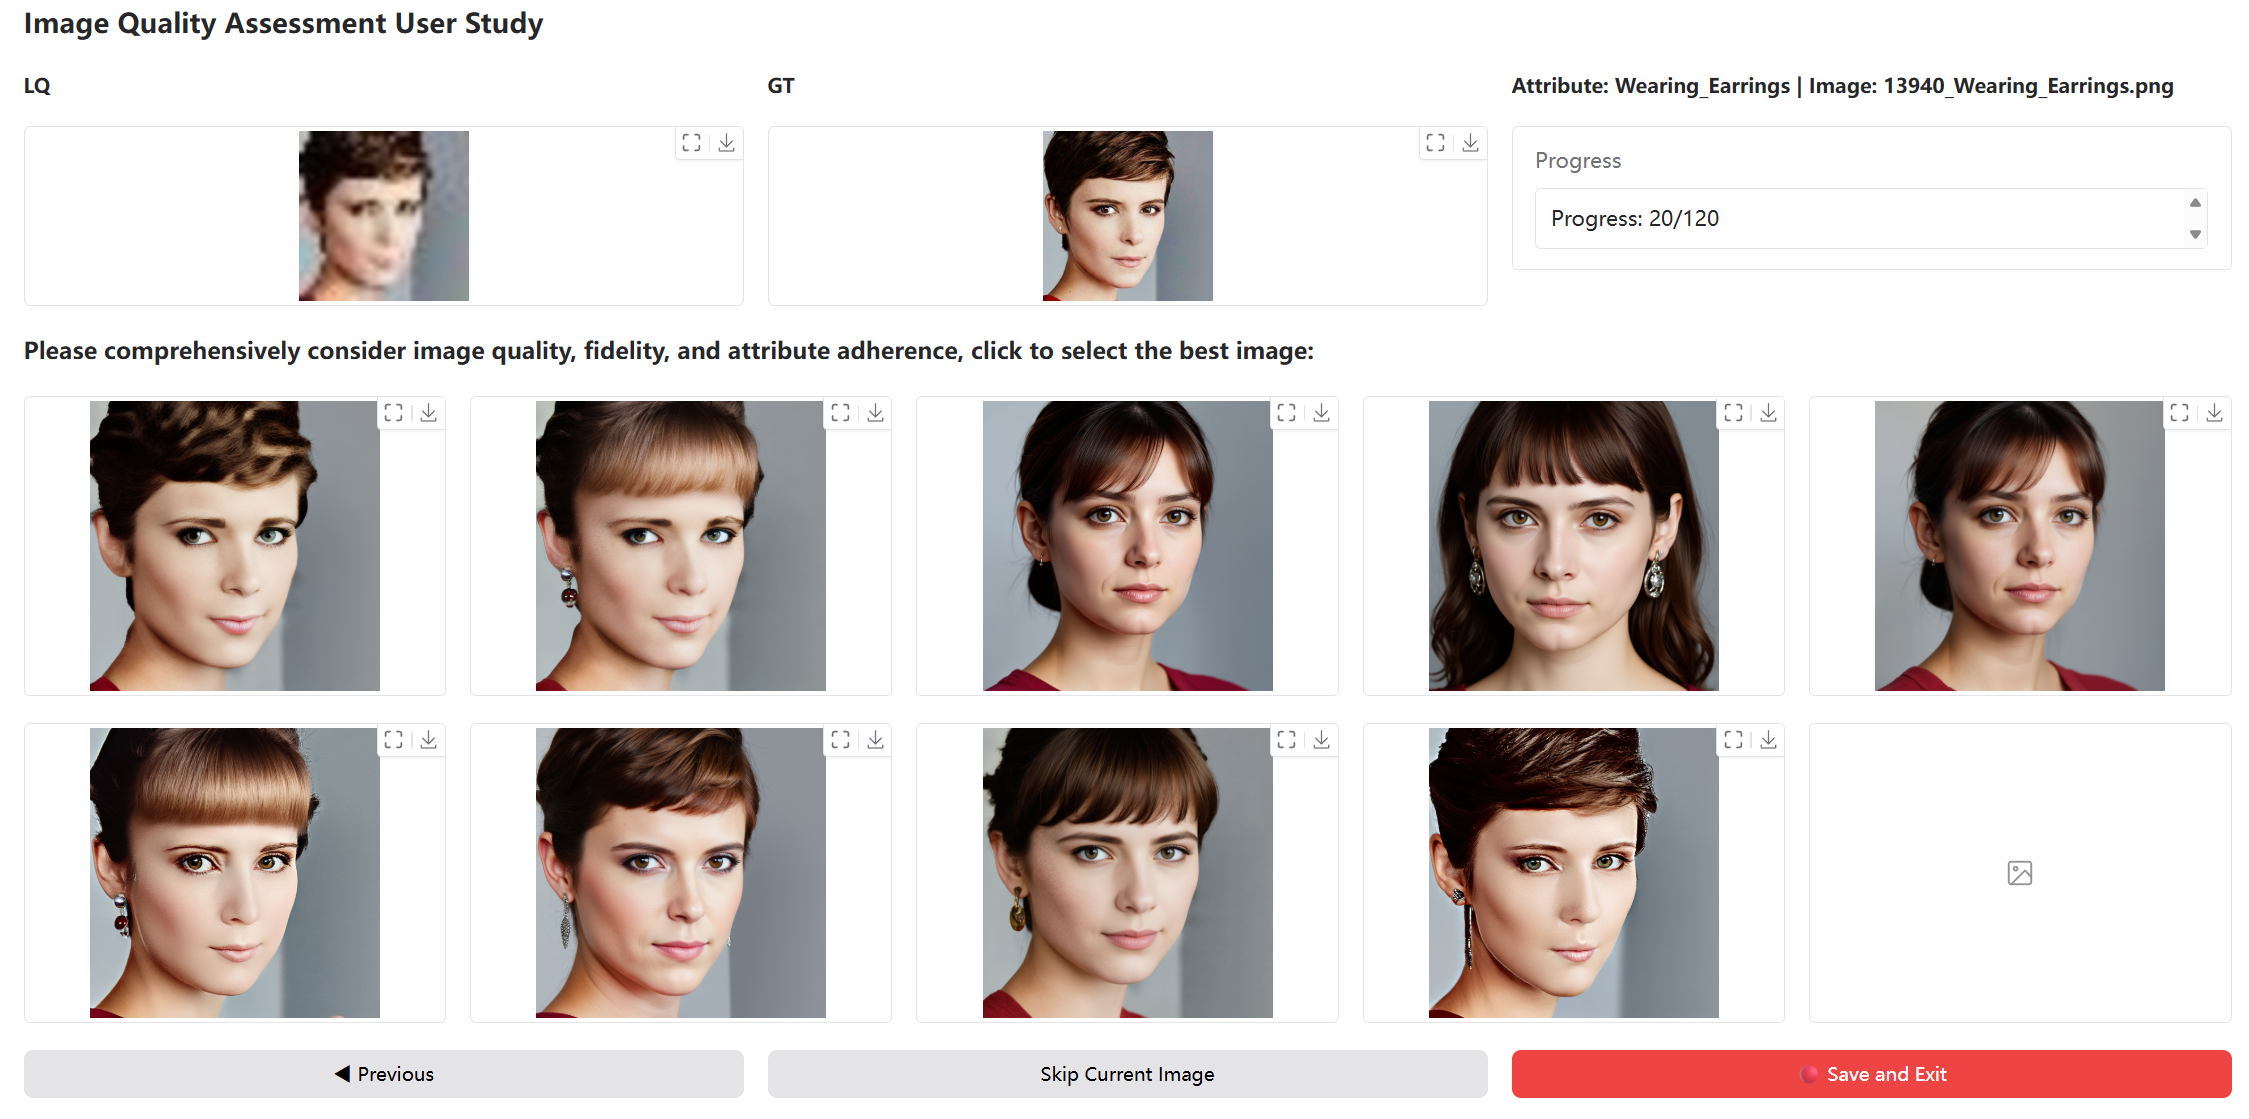}
     \vspace{-8pt}
    \caption{The interface designed for our user study. Participants are required to comprehensively evaluate image quality, fidelity, and attribute adherence to identify the optimal image. }
    \label{fig:user}
     \vspace{-8pt}
\end{figure*}
\begin{figure}[htbp]
    \centering
    \includegraphics[width=0.66\columnwidth]{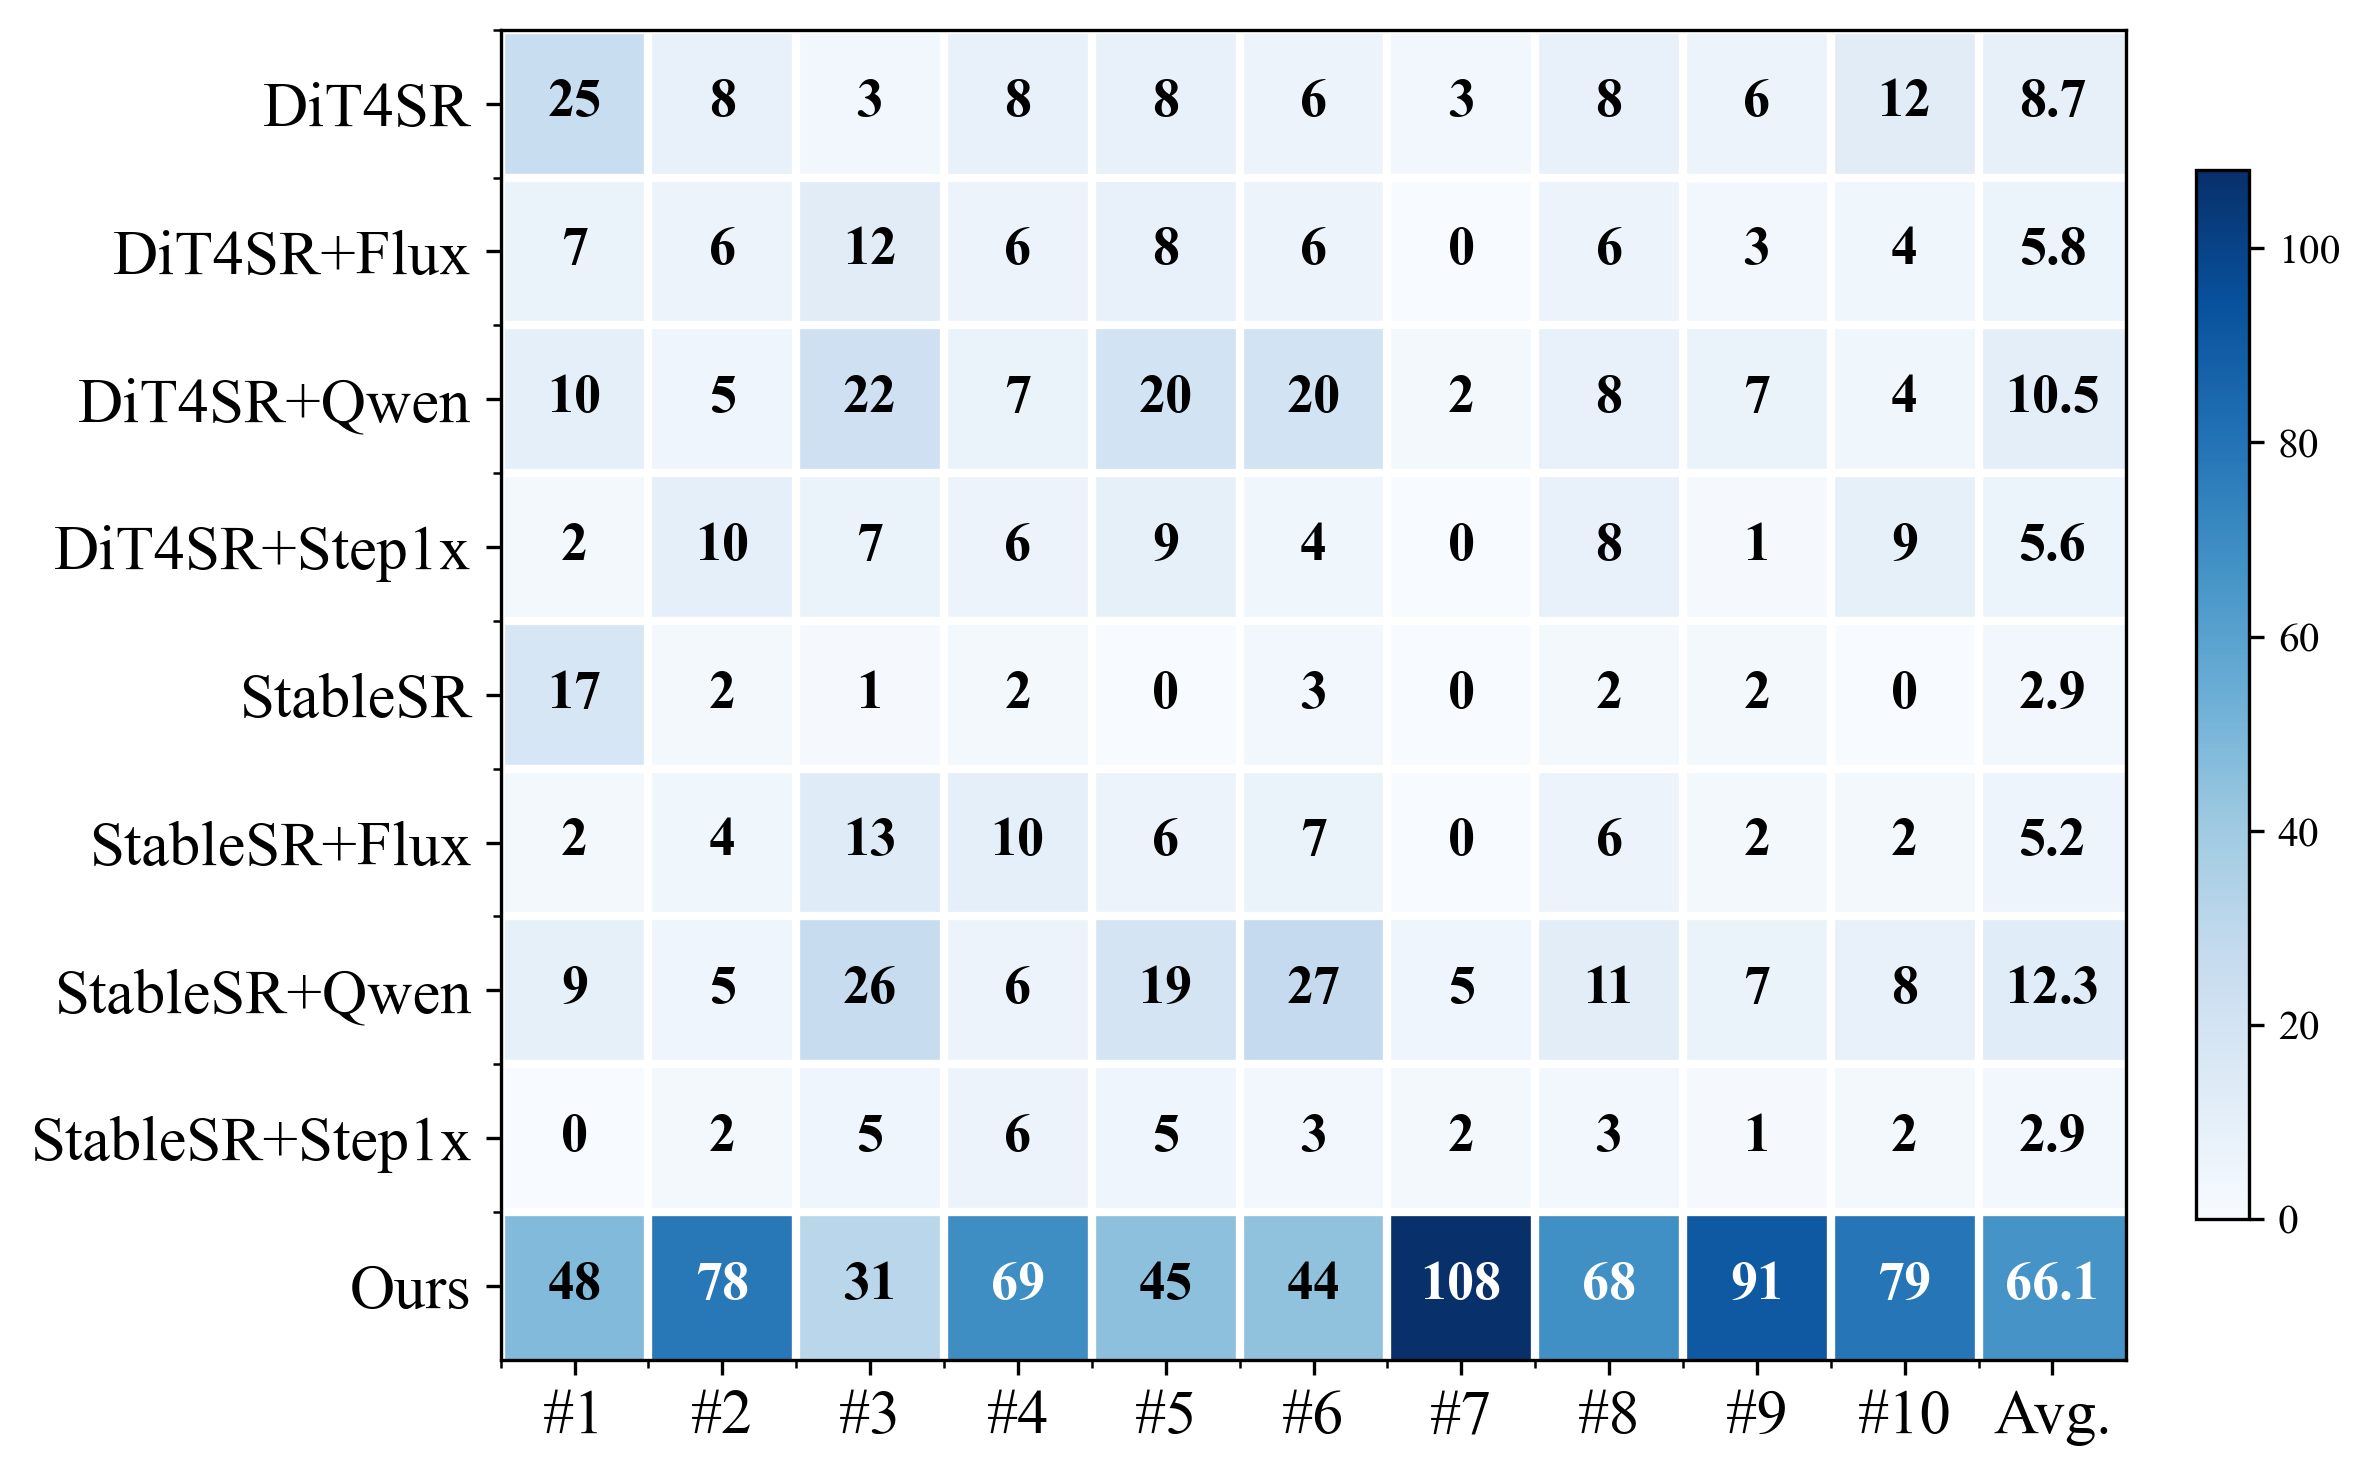}
    \caption{Results of our user study. A total of 10 subjects participated, with \# indicating the subject number. The results further demonstrate \textbf{A$^\text{2}$BFR}'s capacity to balance restoration quality, fidelity, and attribute alignment, surpassing both traditional restoration methods and the restore-then-edit pipeline.}
    \label{fig:user_re}
    \vspace{-12pt}
\end{figure}
\label{sec:userstudy}
% To effectively assess the Attribute-Aware restoration performance of different models, we recruited ten volunteers for our user study. We randomly sampled 120 image sets (10 for each attribute), each comprising the LQ image, GT image, and the outputs of eight different methods and our method. The interface of our user study is shown in Figure~\ref{fig:user}. Each participant is required to comprehensively evaluate image quality, fidelity, and attribute adherence to identify the optimal image. The results are shown in Figure~\ref{fig:user_re}. The results of our user study exhibit a trend consistent with the quantitative findings, further highlighting the significant superiority of our method.

To assess the attribute-aware restoration performance of different methods, we conducted a user study with ten volunteers. We randomly sampled 120 image sets (10 for each attribute), and each set contained the LQ input, the GT image, and the outputs of eight baseline methods together with our method. To reduce presentation bias, the method order in each image set was randomized, and participants were blind to the method identities. Each participant was asked to independently evaluate image quality, fidelity, and attribute adherence, and then select the overall best result for each set. The interface of the user study is shown in Figure~\ref{fig:user}, and the aggregated results are presented in Figure~\ref{fig:user_re}. The preference trend is highly consistent across subjects and aligns well with the quantitative results, further supporting the effectiveness of our method.

\section{Additional Qualitative Results }
\label{sec:qualitative}
\subsection{Responsiveness of Attribute Prompts}
To demonstrate the controllability and attribute responsiveness of \textbf{A$^\text{2}$BFR}, we conduct two separate restoration processes on the same low-quality (LQ) input image: one using a generic template prompt without explicit facial attribute descriptions, and the other using a prompt conditioned on specific facial attributes. The resulting outputs are then compared side by side, clearly showing that \textbf{A$^\text{2}$BFR} is capable of producing attribute-aware restoration results in response to user-specified prompts. Comparative examples are presented in Figure~\ref{fig:visual1}. More qualitative results are provided in Figure~\ref{fig:evisual2} and Figure~\ref{fig:evisual3}.

In addition, we further evaluate the model's ability to handle multi-attribute restoration. As shown in Figure~\ref{fig:multi}, when the input prompt contains multiple facial attributes, \textbf{A$^\text{2}$BFR} can simultaneously follow these attribute instructions and generate restoration results that are both visually plausible and semantically consistent with the given descriptions.

\begin{figure*}[htbp]
    \centering
    \includegraphics[width=\textwidth]{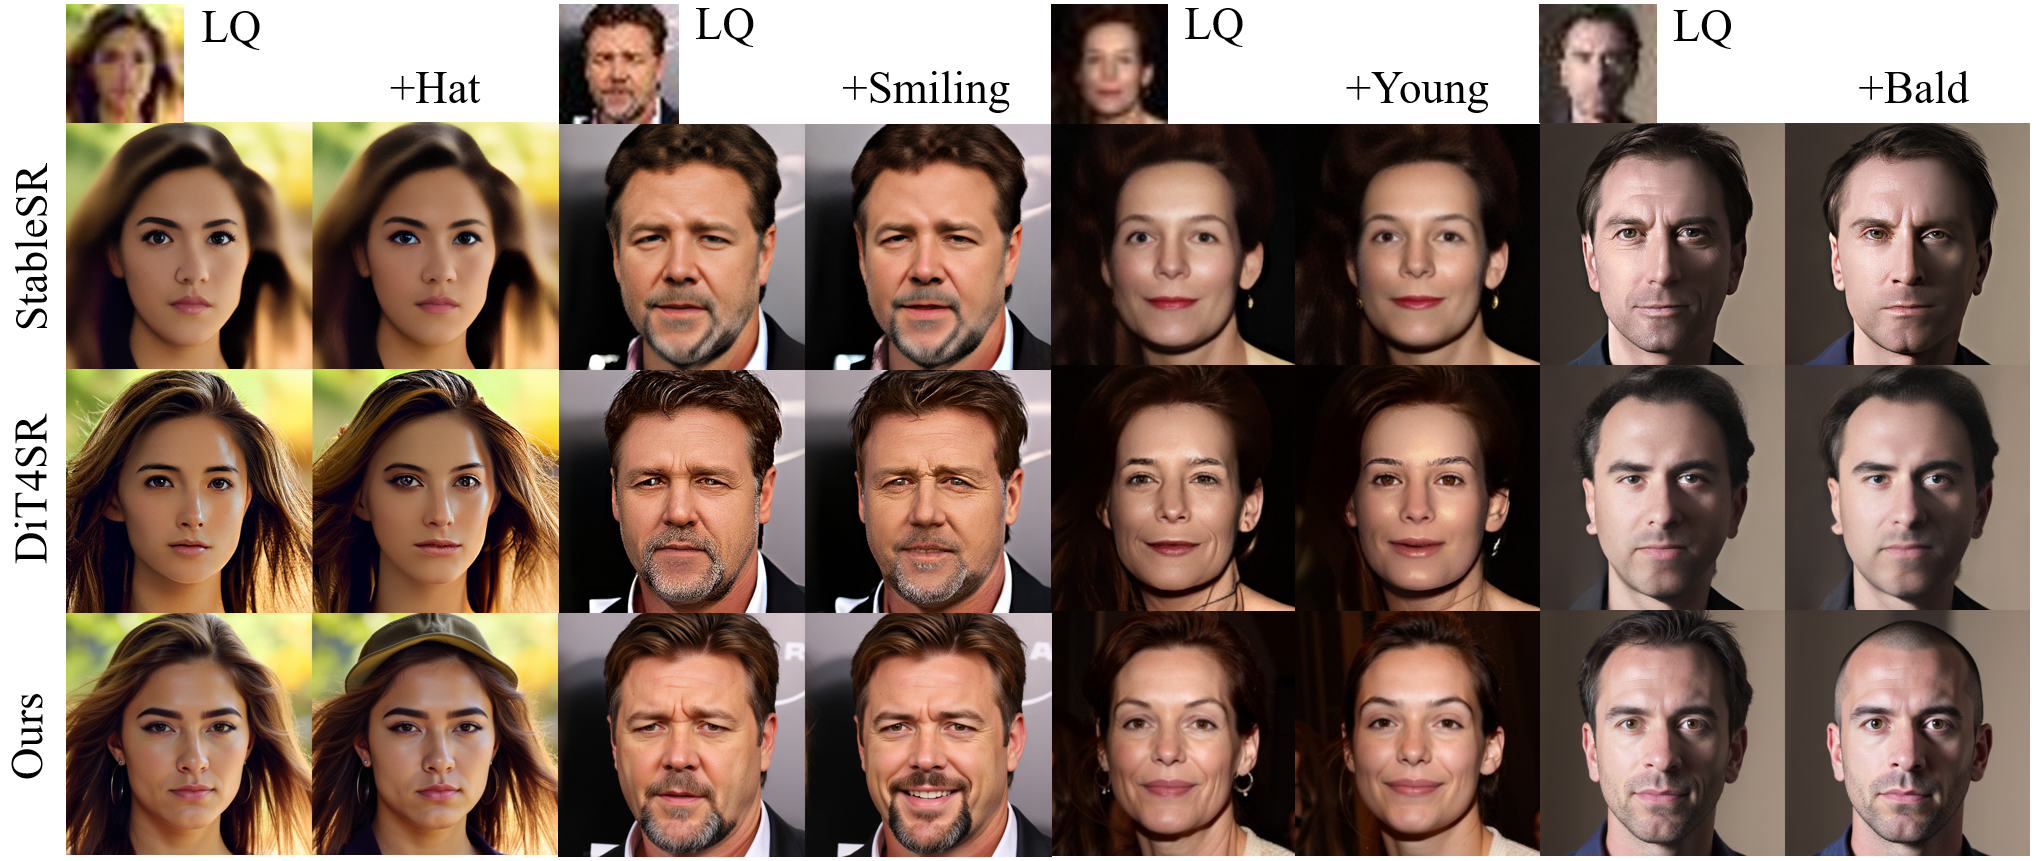}
     \vspace{-8pt}
    \caption{Visual demonstration of the attribute awareness in \textbf{A$^\text{2}$BFR}. The left column shows restoration results using a generic prompt without attribute information, while the right column shows results obtained with an attribute-specific prompt.}
    \vspace{-8pt}
    \label{fig:visual1}
\end{figure*}

\begin{figure*}[htbp]
    \centering
    \includegraphics[width=\textwidth]{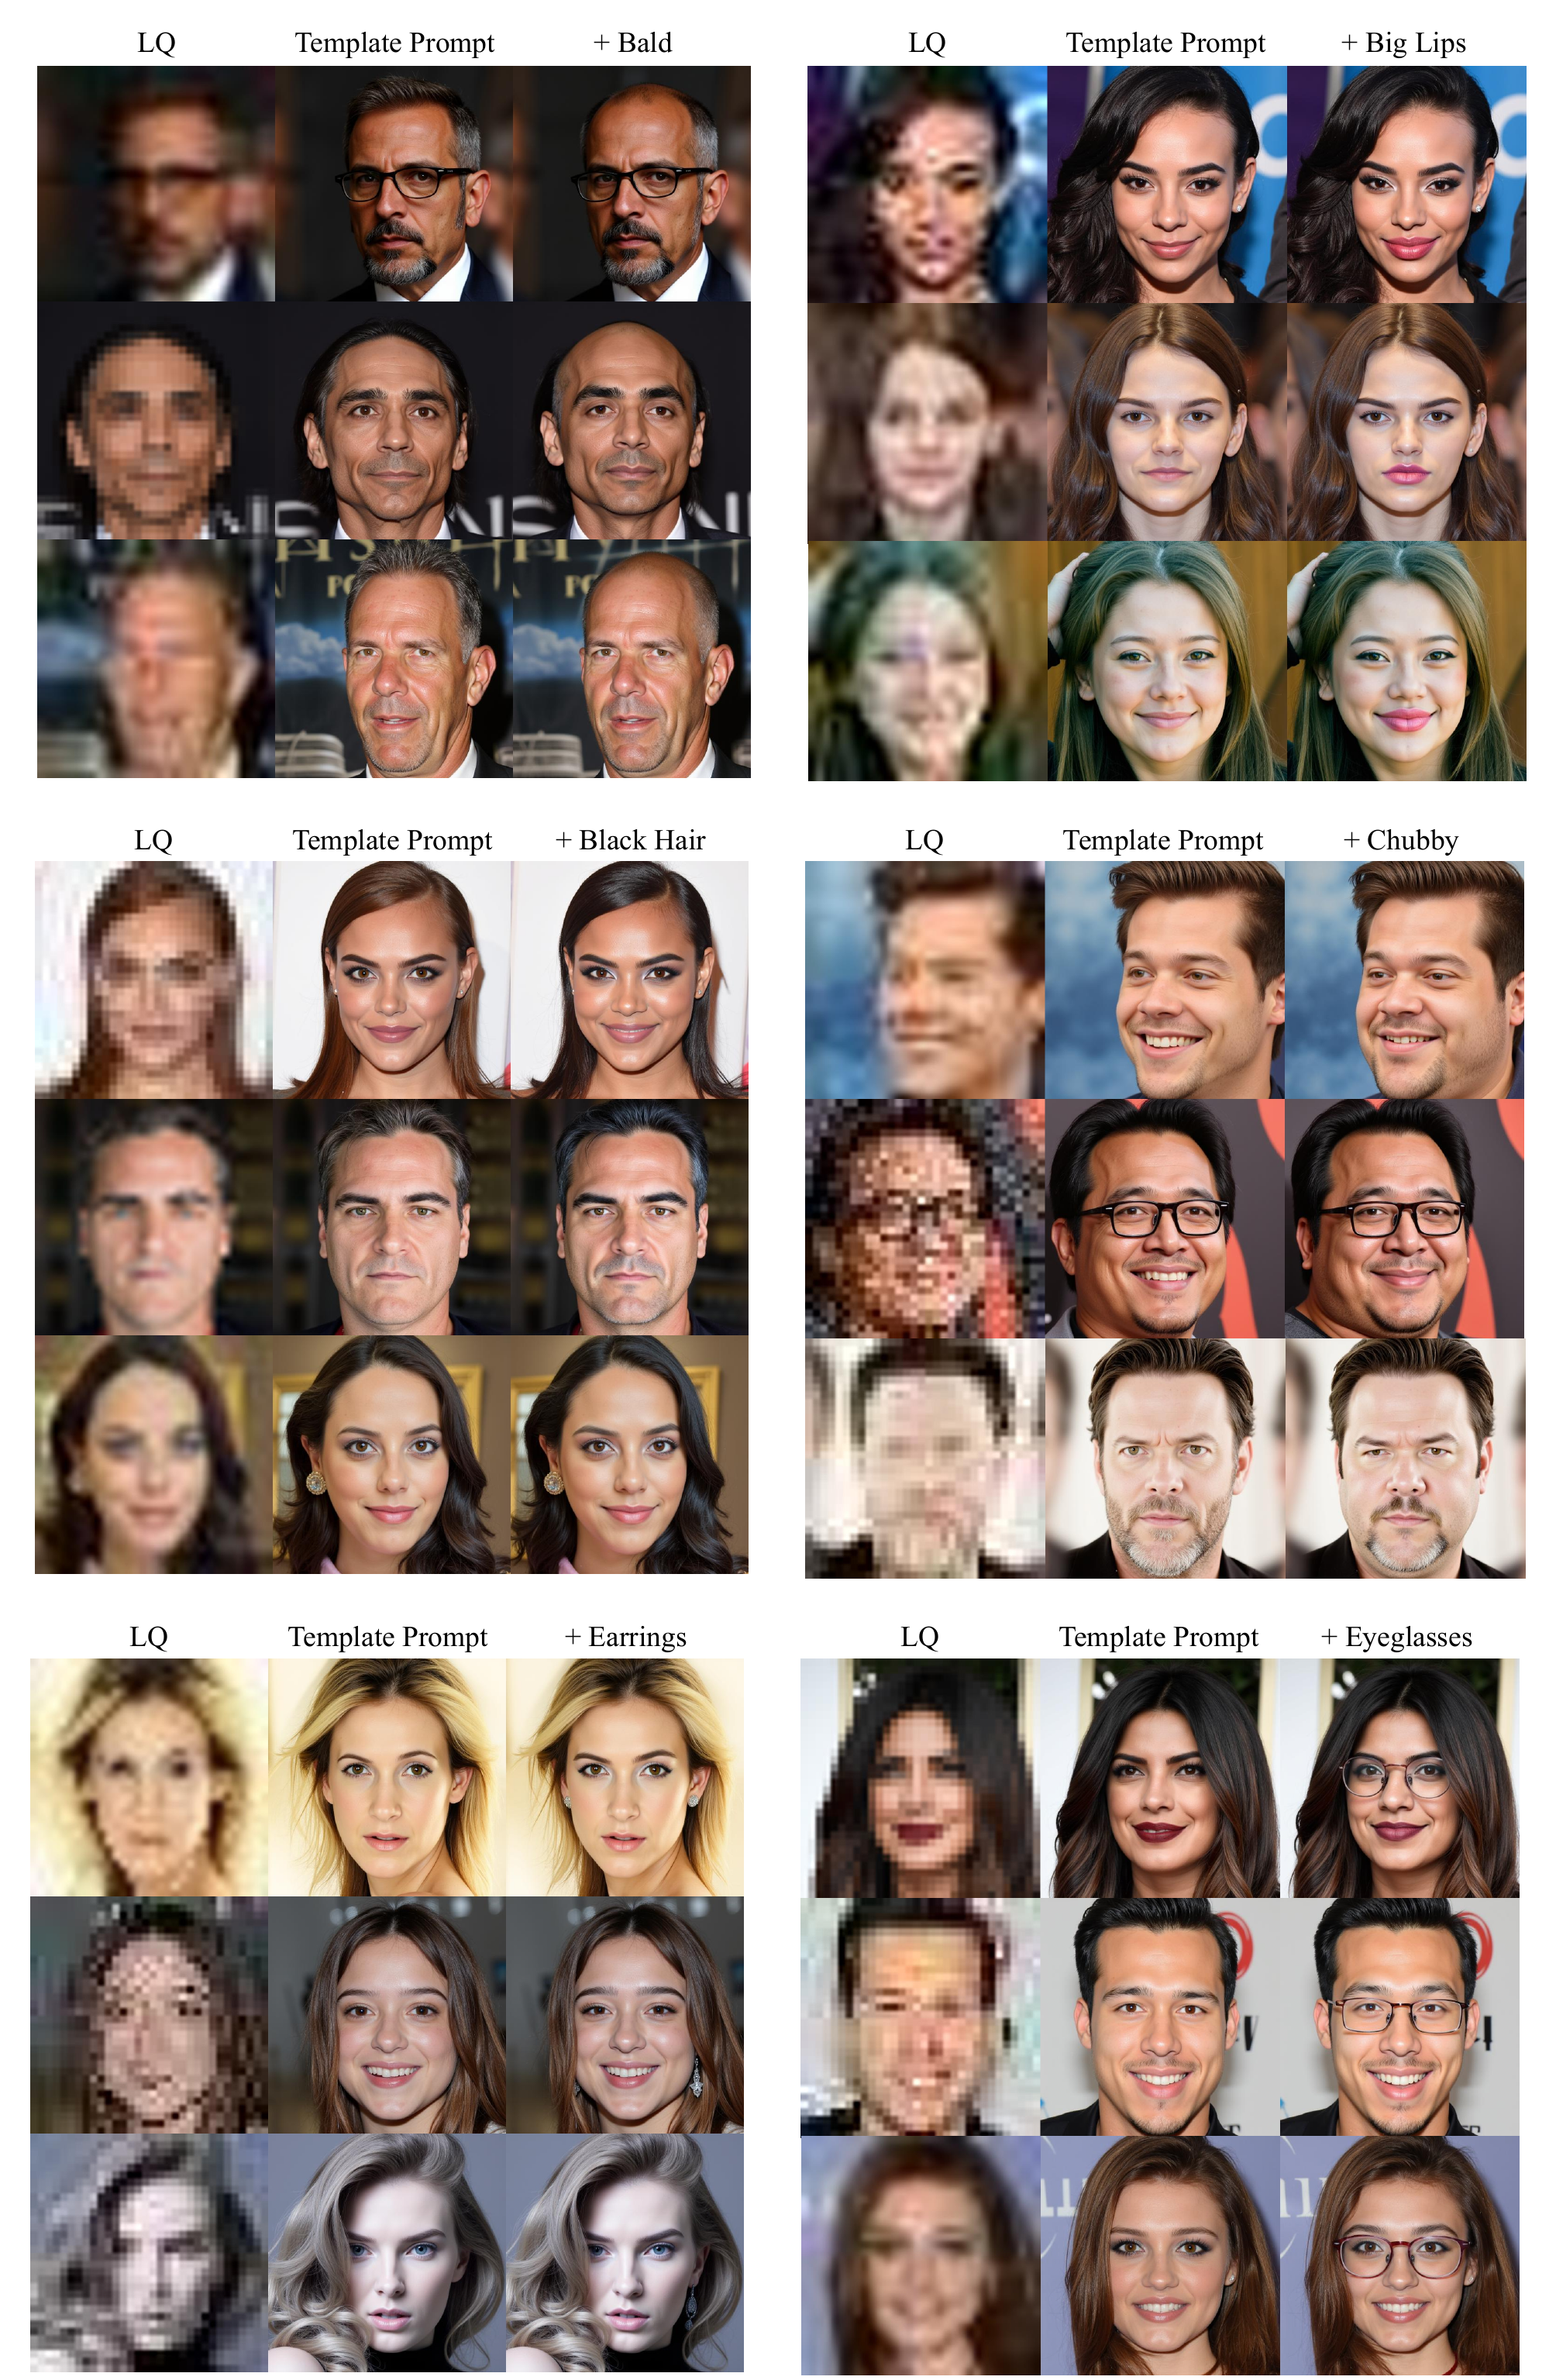}
     \vspace{-16pt}
    \caption{Additional results of \textbf{A$^\text{2}$BFR}. ``Template Prompt'' denotes the prompt ``A photo of a human face.''}
    \label{fig:evisual2}
     \vspace{-8pt}
\end{figure*}

\begin{figure*}[htbp]
    \centering
    \includegraphics[width=\textwidth]{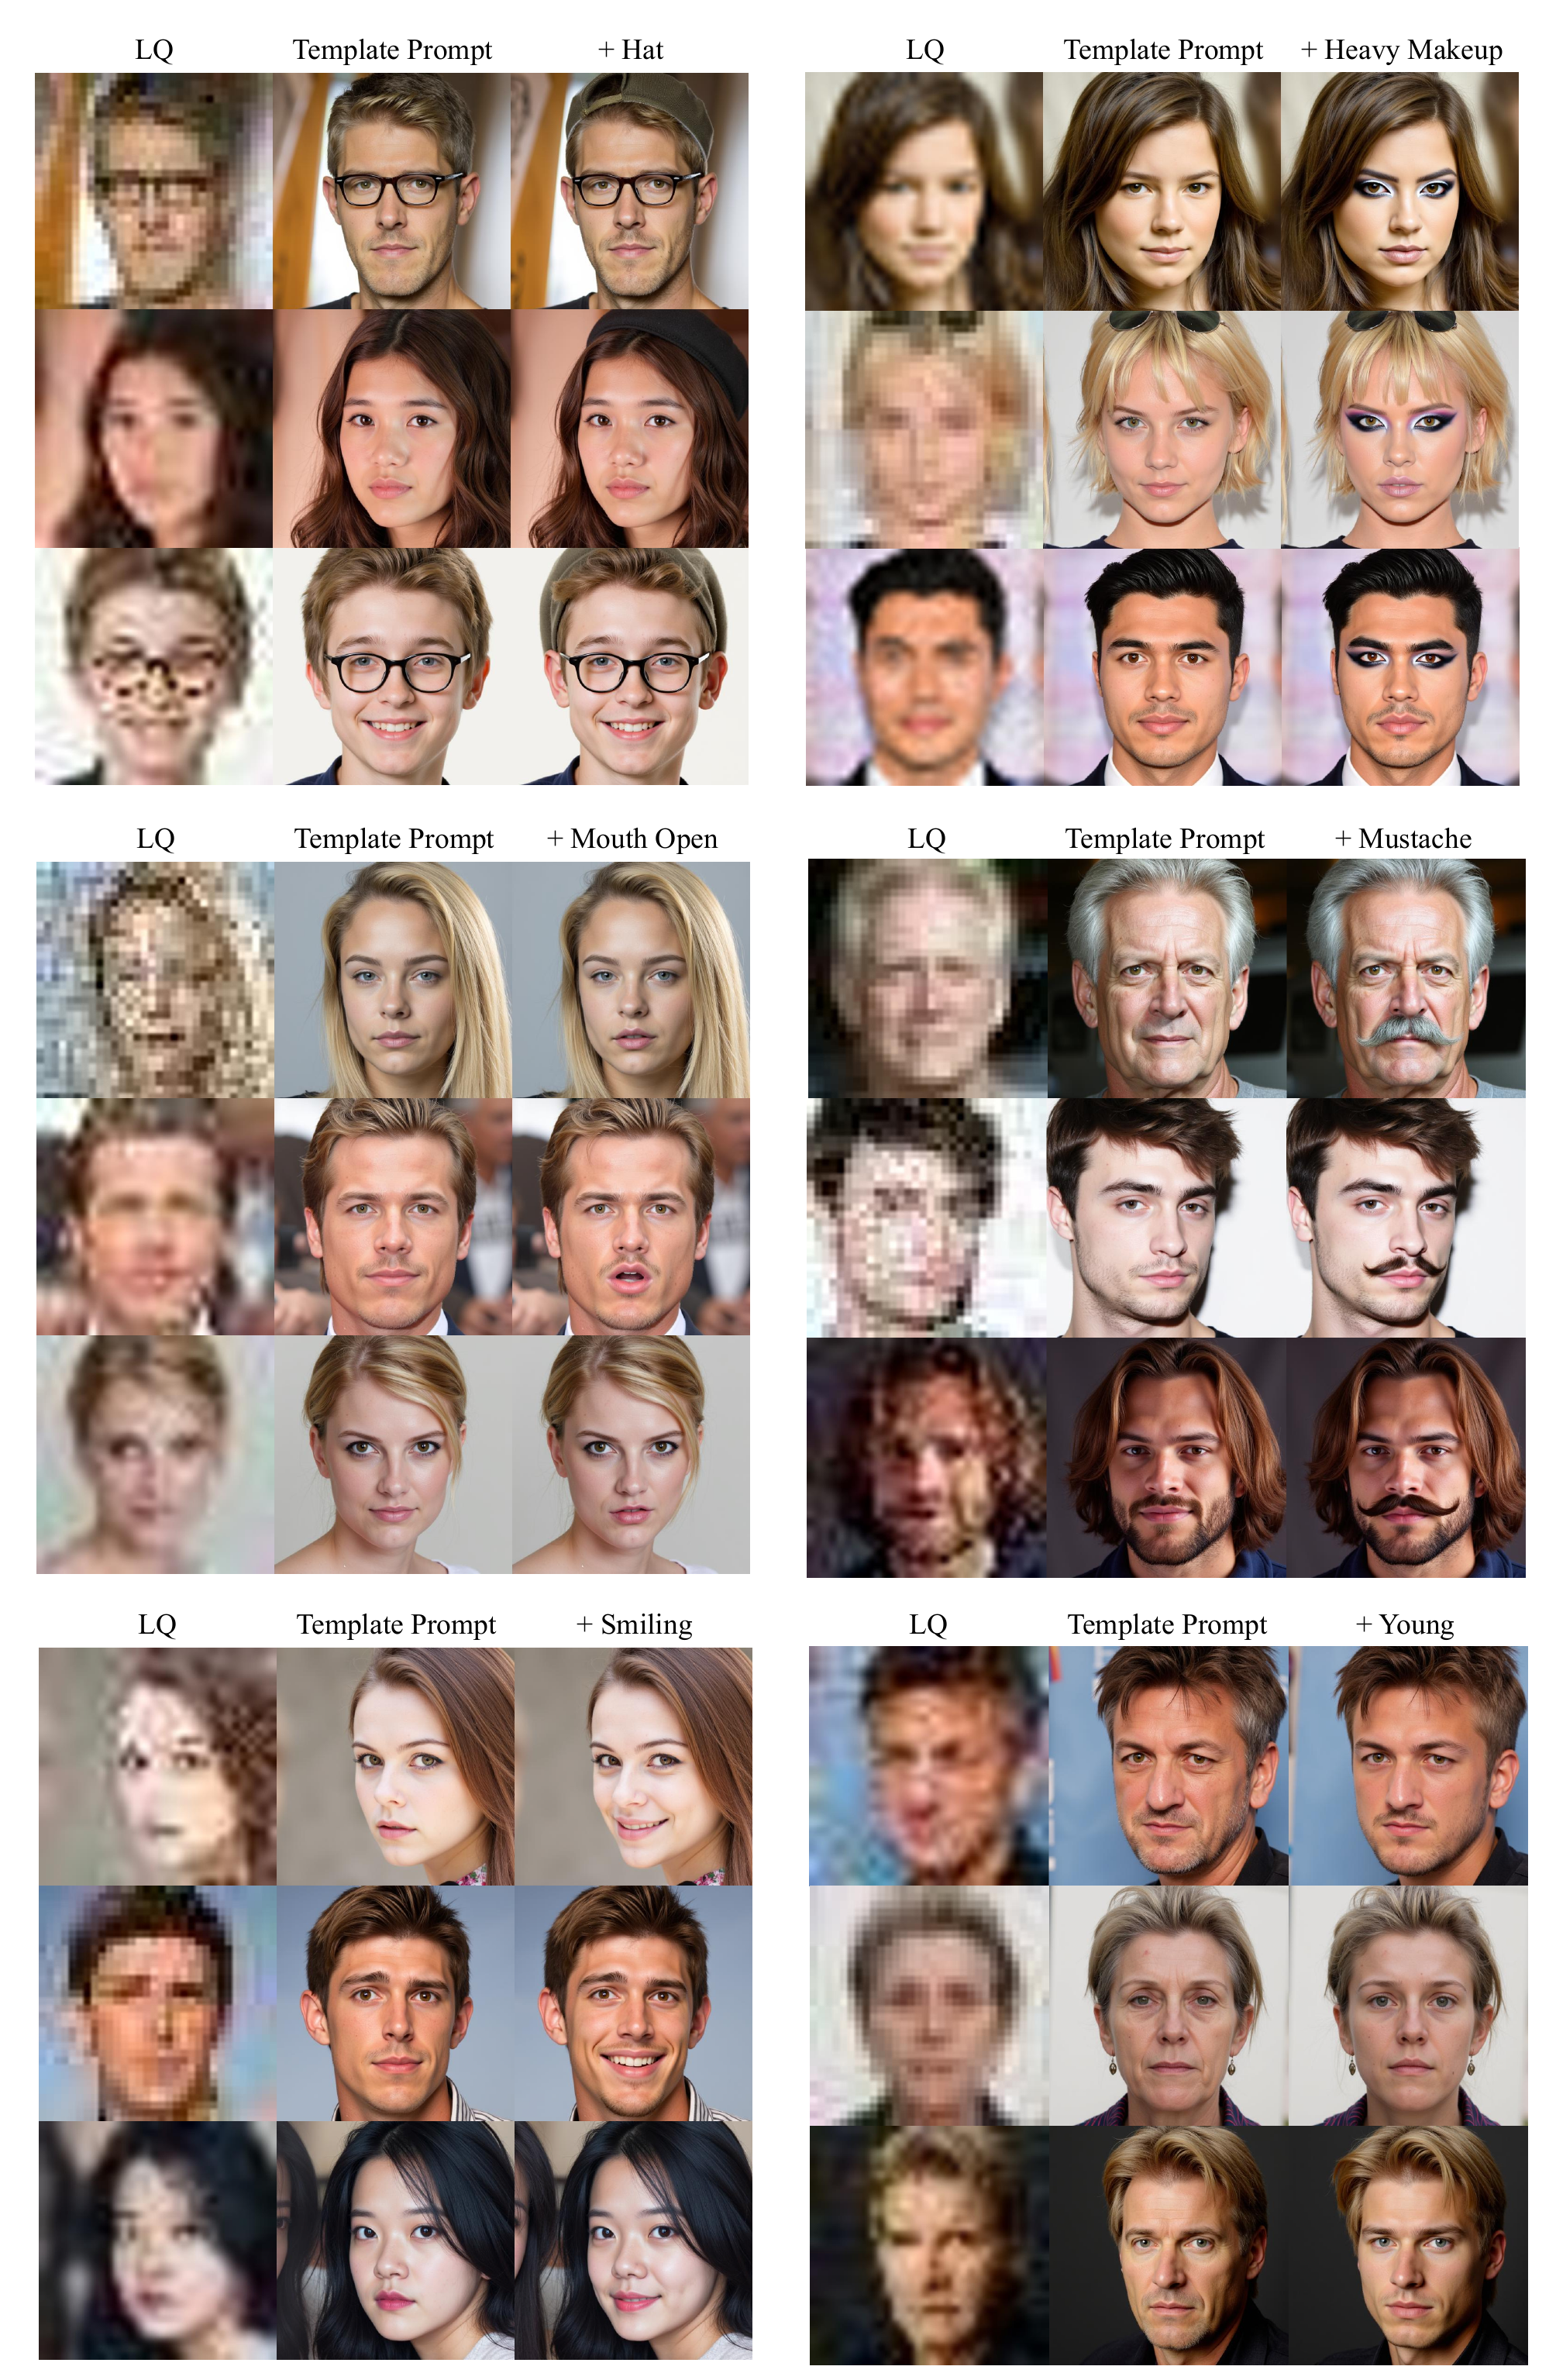}
     \vspace{-16pt}
    \caption{Additional results of \textbf{A$^\text{2}$BFR}. ``Template Prompt'' denotes the prompt ``A photo of a human face.''}
    \label{fig:evisual3}
     \vspace{-8pt}
\end{figure*}

\begin{figure*}[htbp]
    \centering
    \includegraphics[width=\textwidth]{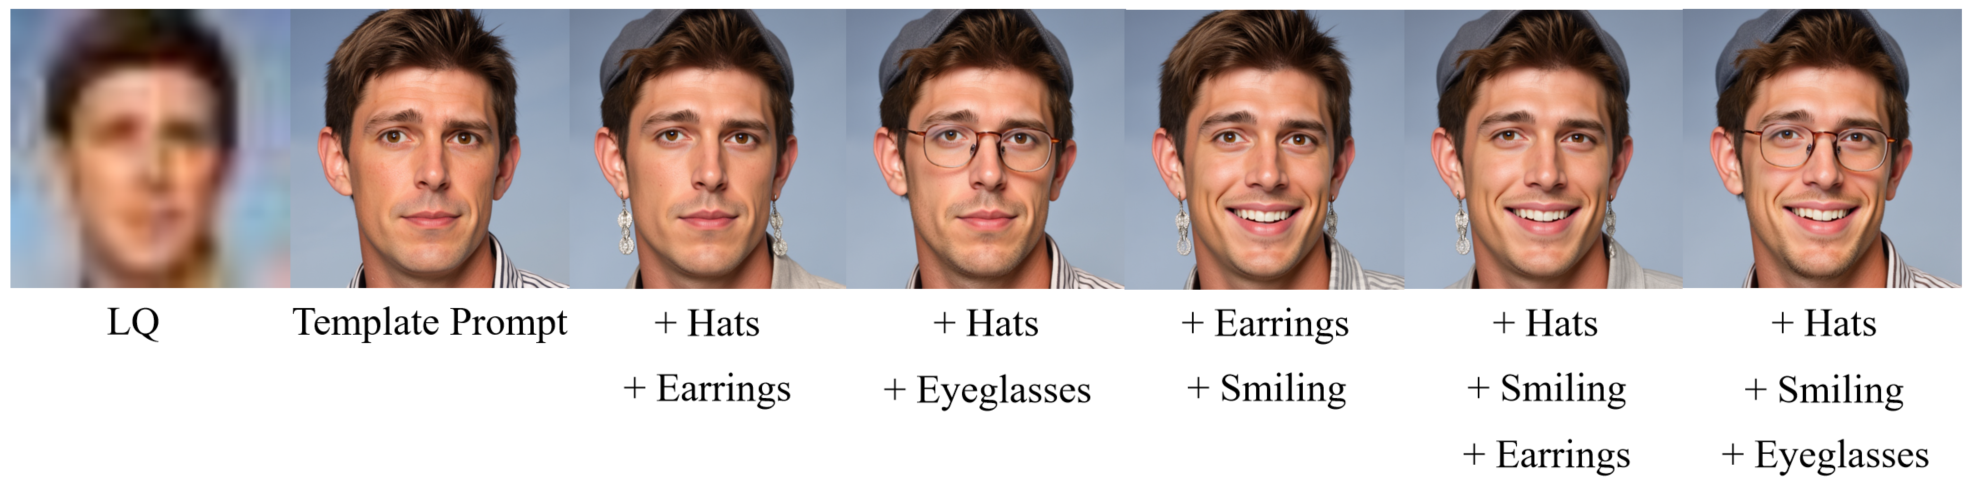}
     \vspace{-8pt}
    \caption{Qualitative results of \textbf{A$^\text{2}$BFR} with multi-attribute prompts. Conditioned on prompts containing multiple facial attributes, \textbf{A$^\text{2}$BFR} produces restored images that faithfully reflect the desired attribute combinations while maintaining realistic facial details and overall visual quality.  }
    \label{fig:multi}
\end{figure*}

\subsection{Model Generalization Capability}
To comprehensively evaluate the generalization ability of our method, we conduct extensive experiments across three challenging scenarios:

\textbf{Different Degradation Levels.}
\textbf{A$^\text{2}$BFR} demonstrates strong robustness across various degradation levels, consistently producing high-quality, artifact-free facial reconstructions even under severe degradation conditions. As shown in Figure~\ref{fig:visual3}, the model maintains highly consistent restoration performance at  $8\times$ and $16\times$ downsampling scales, and continues to generate high-quality facial images even at the challenging $32\times$ restoration level.

\begin{figure}[htbp]
    \centering
    \includegraphics[width=\columnwidth]{pics/dd.png}
    \caption{Qualitative results on different degradation levels. \textbf{A$^\text{2}$BFR} exhibits high robustness to varying degrees of degradation, capable of restoring high-quality, artifact-free face images even under severe degradation conditions.}
    \label{fig:visual3}
\end{figure}

\textbf{Out-of-Domain Attributes.} \textbf{A$^\text{2}$BFR} demonstrates encouraging generalization beyond the 12 attribute categories defined in AttrFace-90K. As shown in Figure~\ref{fig:visual4}, the model can successfully follow out-of-domain prompts, including descriptions such as \textit{``angry''}, \textit{``blue eyes''}, and \textit{``necklace''}. These results indicate that \textbf{A$^\text{2}$BFR} can generalize to unseen semantic descriptions while maintaining semantically coherent and visually plausible restoration results.

\begin{figure}[htbp]
    \centering
    \includegraphics[width=\columnwidth]{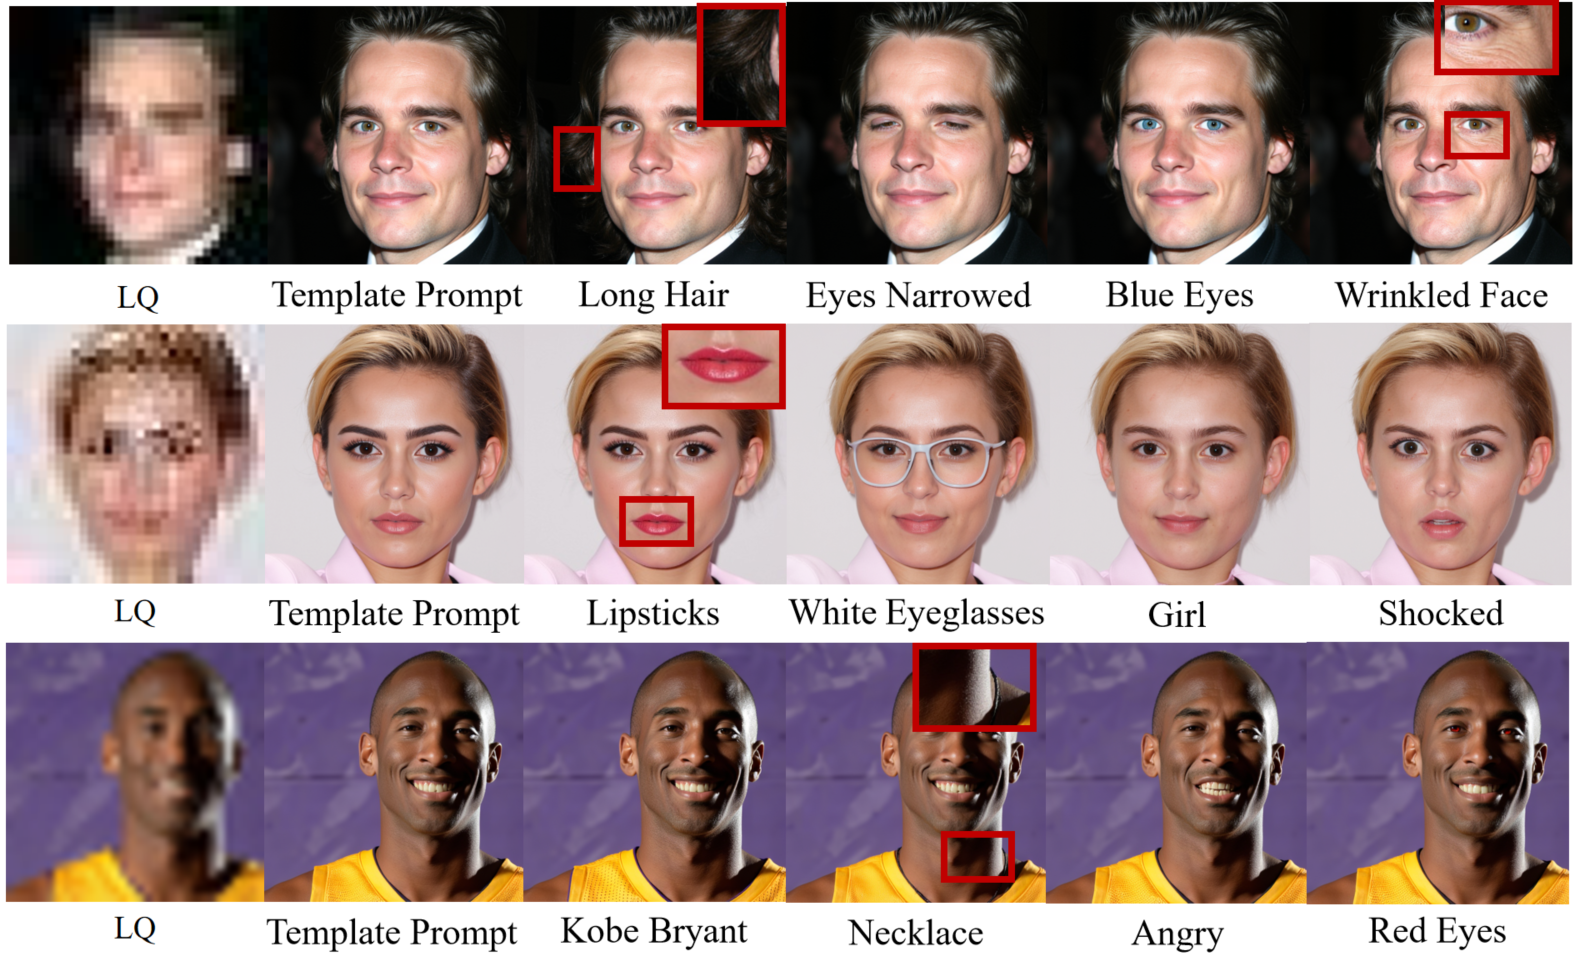}
    \caption{Qualitative results on out-of-domain attributes. \textbf{A$^\text{2}$BFR} remains responsive to attribute prompts beyond the 12 categories defined in AttrFace-90K and generates semantically consistent restoration results.}
    \label{fig:visual4}
\end{figure}

\textbf{Anime Face Restoration.} \textbf{A$^\text{2}$BFR} exhibits notable generalization capability beyond photographic faces, achieving compelling results in anime face restoration tasks. As shown in Figure~\ref{fig:visual5}, without specific training on animated content, the model effectively preserves distinctive artistic styles while enhancing resolution and reducing artifacts, demonstrating its adaptability to diverse facial representation domains.

\begin{figure}[htbp]
    \centering
    \includegraphics[width=\columnwidth]{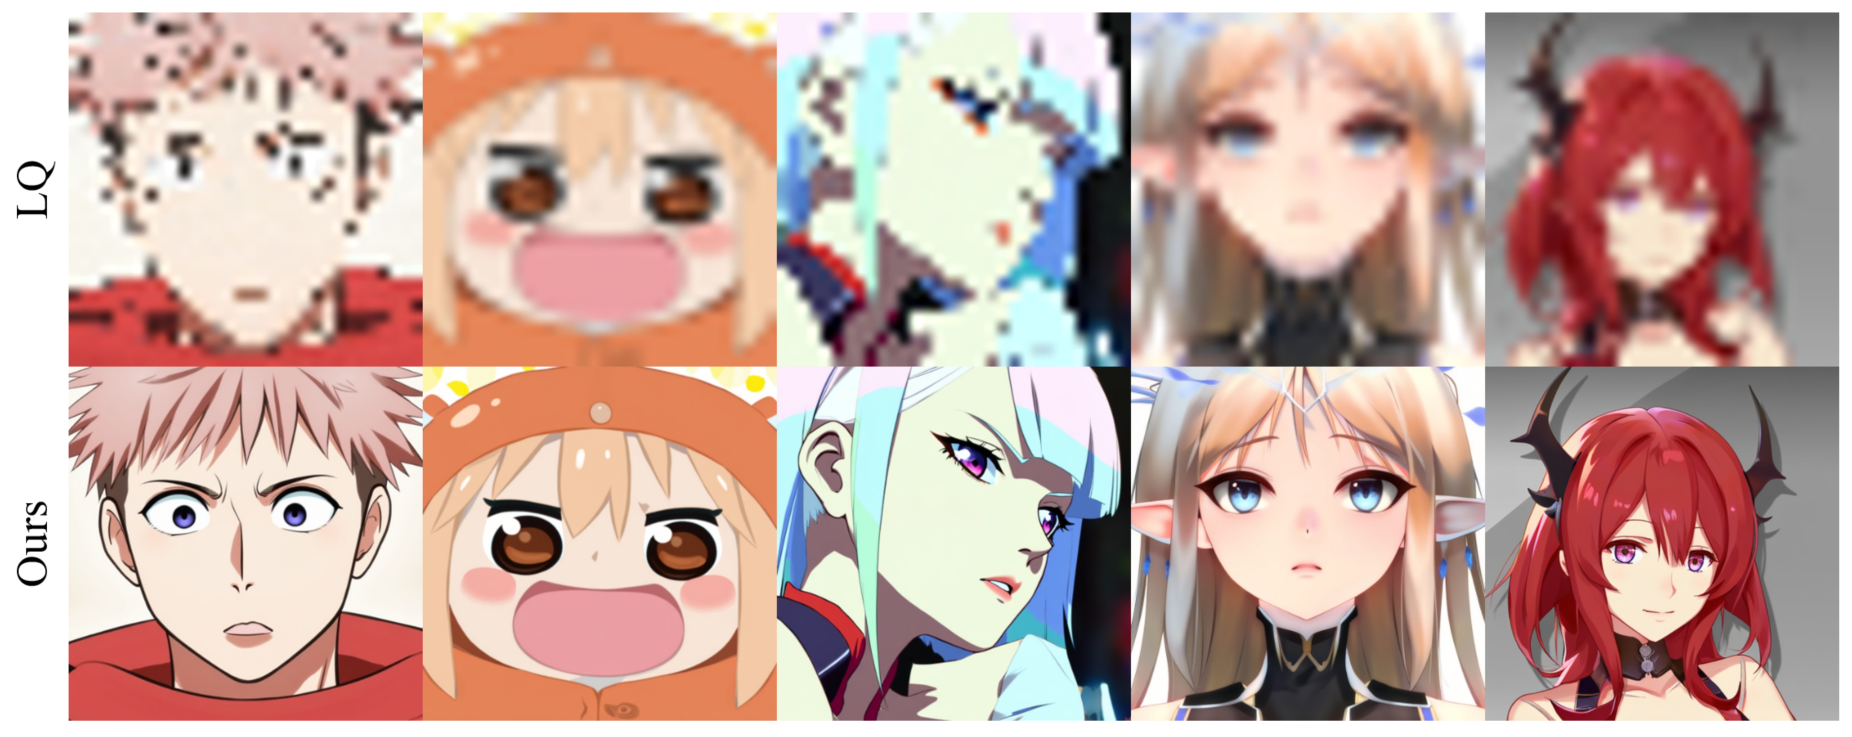}
    \caption{Qualitative results of Anime Face Restoration. \textbf{A$^\text{2}$BFR} demonstrates strong generalization capability, achieving robust performance in anime face restoration tasks.}
    \label{fig:visual5}
\end{figure}

Overall, these results suggest that \textbf{A$^\text{2}$BFR} exhibits promising generalization ability across multiple scenarios. The model remains effective under varying degradation levels, can follow unseen semantic descriptions beyond the predefined attribute categories, and shows encouraging transferability to anime faces. These observations indicate that \textbf{A$^\text{2}$BFR} learns a relatively flexible restoration prior, enabling both high-quality reconstruction and controllable semantic adaptation beyond the training distribution.

\section{Limitations}
\label{sec:limitation}
First, we are fully cognizant of and attentive to privacy concerns associated with facial datasets. All raw data are derived exclusively from existing open-source datasets, and both collection and sharing processes strictly adhere to relevant privacy policies. Second, the proposed AttrFace-90K dataset contains face image pairs varying across 12 predefined attributes, and we hope to expand the attribute diversity in our dataset for future work.
